# Supplementary material for: Learning in Markov Decision Processes under Constraints
Source: arXiv:2002.12435 source file (2022-01-05)
Supplement: Supplementary file 1 [file Supplement.pdf]

---

# Learning in Constrained Markov Decision Processes

---

Anonymous Author(s)

Affiliation

Address

email

## Abstract

We consider reinforcement learning (RL) in Markov Decision Processes in which an agent repeatedly interacts with an environment that is modeled by a controlled Markov process. At each time step  $t$ , it earns a reward, and also incurs a cost-vector consisting of  $M$  costs. We design learning algorithms that maximize the cumulative reward earned over a time horizon of  $T$  time-steps, while simultaneously ensuring that the average values of the  $M$  cost expenditures are bounded by agent-specified thresholds  $c_i^{ub}, i = 1, 2, \dots, M$ . The considerations on the cumulative cost expenditures is in departure from the existing literature, in that the agent now additionally needs to balance the cost expenses in an online manner, while simultaneously performing the exploration-exploitation trade-off that is typically encountered in RL tasks. This is challenging since the duo objectives of exploration and exploitation necessarily require the agent to expend resources. Since learning algorithms such as UCRL2 that are based on the principle of optimism in the face of uncertainty might be infeasible, we modify it appropriately and propose UCRL-CMDP algorithm.

In order to measure the performance of a reinforcement learning algorithm that satisfies the average cost constraints, we define an  $M + 1$  dimensional regret vector that is composed of its reward regret, and  $M$  cost regrets. The reward regret measures the sub-optimality in the cumulative reward, while the  $i$ -th component of the cost regret vector is difference between its  $i$ -th cumulative cost expense and the expected cost expenditures  $Tc_i^{ub}$ . We prove that with a high probability, the regret vector of UCRL-CMDP is upper-bounded as  $O\left(S\sqrt{AT^{1.5}\log(T)}\right)$ , where  $S$  is the number of states,  $A$  is the number of actions, and  $T$  is the time horizon. We further show how to reduce the regret of a desired subset of the  $M$  costs, at the expense of increasing the regrets of rewards and the remaining costs.

## 1 Introduction

Reinforcement Learning (RL) [SB98] involves an agent repeatedly interacting with an environment modelled by a Markov Decision Process (MDP) [Put14] that is characterized by its state-space  $\mathcal{S}$ , action-space  $\mathcal{A}$  and controlled transition probabilities  $\{p(s, a, s')\}_{s, s' \in \mathcal{S}, a \in \mathcal{A}}$ . At each discrete time  $t = 1, 2, \dots, T$ , the agent observes the current state of the environment  $s_t$ , applies control  $a_t$ , and earns a reward  $r_t$  that is a known function of  $(s_t, a_t)$ . The agent does not know the controlled transition probabilities  $p(s, a, s')$  that describe the system dynamics of the environment. The performance of the agent is measured by the cumulative rewards that it earns over the time horizon.

In many applications, in addition to earning rewards, the agent also incurs costs at each time. The underlying physical constraints impose constraints on its cumulative cost expenditures, so that the agent needs to balance its reward earnings with the cost accretion while also simultaneously learning the choice of optimal decisions, all in an *online manner*.

As a motivating example, consider a single-hop wireless network that consists of a wireless node that transmits data packets to a receiver over an unreliable wireless channel. The channel reliability, i.e., the probability that a transmission at time-step  $t$  is successful, depends upon the instantaneous channel state  $cs_t$  and the transmission power  $a_t$ . Thus, for example, this probability is higher when the channel is in a good state, or if transmission is carried out at higher power levels. The transmitter stores packets in a buffer, and its queue-length at time  $t$  is denoted by  $Q_t$ . It has to choose  $a_t$  adaptively so as to minimize the average queue length  $(\mathbb{E} \sum_{t=1}^T Q_t) / T$ ; which is an appropriate performance metric [Sen09]. In this example, the state of the “environment” at time  $t$  is given by the queue-length and the channel state  $(Q_t, cs_t)$ . Since the wireless node is battery-operated, its average power consumption has to be less than its capacity  $c^{ub}$ , i.e.,  $(\mathbb{E} \sum_{t=1}^T a_t) / T \leq c^{ub}$ , where the quantity  $c^{ub}$  is calculated on the basis of the expected lifetime of the wireless node, and the total electric charge that it can hold. Thus, it might be “optimal” to utilize high transmission power levels only in the case when the instantaneous queue length  $Q_t$  is large or the wireless channel’s state  $cs_t$  is good; this strategy saves energy by transmitting at lower energy levels at other times.

Since channel reliabilities are typically not known to the transmitter node, it does not know the transition probabilities  $p(s, a, s')$  that describe the controlled process  $(Q_t, cs_t)$ . Hence, it cannot compute the expectations of the average queue lengths and average power consumption for a fixed control policy, and needs to devise appropriate learning policies to optimize its performance under average-cost constraints. RL algorithms that we propose in this work solve exactly these classes of problems.

## 1.1 Previous Works

**RL Algorithms for unconstrained MDPs:** RL problems without constraints are well-understood by now. Works such as [BT02, AO07, BT09, JOA10] develop algorithms using the principle of “optimism under uncertainty.” UCRL2 of [JOA10] is a popular RL algorithm that has a regret bound of  $\tilde{O}(D(p)S\sqrt{AT})$ , where  $D(p)$  is the diameter of the MDP  $p$  (see (1)); the algorithms proposed in our work are based on UCRL2.

**RL Algorithms for Constrained MDPs:** [AS91] is an early work on optimally controlling unknown MDPs under average cost constraints. It utilizes the certainty equivalence (CE) principle, i.e., it applies controls that are optimal under the assumption that the true (but unknown) MDP parameters are equal to the empirical estimates, and also occasionally resorts to “forced explorations.” This algorithm yields asymptotically (as  $T \rightarrow \infty$ ) the same reward rate as the case when the MDP parameters are known. However, analysis is performed under the assumption that the CMDP is *strictly feasible*, and moreover the algorithm lacks finite-time performance guarantees (bounds on regret). Unlike [AS91], we do not assume strict feasibility; infact we show that the use of *confidence bounds* allows us to rid the strict feasibility assumption.

Another work [Bor05] derives a learning scheme based on multi time-scale stochastic approximation [Bor97], in which the task of learning optimal policy for the CMDP is decomposed into that of learning the optimal value of the dual variables, which correspond to the price of violating the average cost constraints, and that of learning the optimal policy for an unconstrained MDP parameterized by the dual variables. However, the proposed scheme lacks finite-time regret analysis, and might suffer from a large regret. Prima facie, this layered decomposition might not be optimal with respect to the sample-complexity of the online RL problem.

**Bandit Algorithms under Budget Constraints:** A somewhat related problem called the multi-armed bandits (MAB) under budget constraints has been studied in the MAB literature [BKS18, BKS13, DQZL13, CJS15]. In the classical MAB problem, the learner has to pull one out of  $K$  arms at each discrete time step. Pulling an arm yields a (random) reward, whose distribution depends upon the choice of arm. The learner has to sequentially pull arms so as to maximize the expected value of the cumulative rewards earned over a time period. In MAB under budget constraints, pulling an arm also incurs a random cost, and the probability distributions governing the instantaneous rewards and costs are a function of chosen arm. The agent can spend a maximum of  $B$  units of resources, and has to pull the arms so as to maximize the cumulative rewards earned until the time when the resources are exhausted. Our set-up differs from the budgeted MAB problem since unlike the MAB,

in which there is no notion of environment’s state, the evolution of the state of the underlying MDP in our setup introduces temporal correlations in the reward and the  $M$  cost processes.

## 1.2 Contributions

Our contributions are summarized as follows.

1. We initiate the problem of designing RL algorithms that maximize the cumulative rewards while simultaneously satisfying average cost constraints. We propose an algorithm which we call UCRL for CMDPs, henceforth abbreviated as UCRL-CMDP. UCRL-CMDP is a modification of the popular RL algorithm UCRL2 of [JOA10] that utilizes the principle of optimism in the face of uncertainty (OFU) while making decisions. Since an algorithm that utilizes OFU need not satisfy cost constraints (this is discussed briefly below by presenting an example), we modify OFU appropriately and derive the principle of *balanced optimism in the face of uncertainty* (BOFU). Under the BOFU principle, at the beginning of each “RL” episode, the agent has to solve for (i) an MDP, and (ii) a controller, such that the average costs of a system in which the dynamics are described by (i), and which is controlled using (ii), are less than or equal to the cost constraints.
2. We show that the use of BOFU allows us to overcome the shortcomings of CE approach that were encountered in [AS91], i.e., there are arbitrarily long time-durations during which the CMDP in which the system dynamics are described by the current empirical estimates of transition probabilities is infeasible, and hence the agent is unable to utilize these estimates in order to make control decisions. As a by-product, BOFU also allows us to get rid of “forced explorations,” that were utilized in [AS91], i.e., employing randomized controls occasionally.
3. In order to quantify the finite-time performance of a RL algorithm that has to perform under average cost constraints, we define its  $M + 1$ -dimensional “regret vector” that is composed of its reward regret and  $M$  cost regrets. More precisely, considering solely the reward regret (as is done in the RL literature) overlooks the cost expenditures. Indeed, we show that the reward regret can be made arbitrary small (with a high probability) at the expense of an increase in the cumulative cost expenditure. Thus, while comparing the performance of two different learning algorithms, we also need to compare their cost expenditures. Reward regret of a learning algorithm is the difference between its reward and the reward of an optimal policy that knows the MDP parameters, while the  $i$ -th cost regret is the difference between the total cost incurred until  $T$  time-steps, and  $c_i^{ub}T$ . Analogous to the unconstrained RL setup, in which one is interested in quantifying a lower bound on the regret of any learning algorithm, we ask the following question in the constrained setup: *What is the set of “achievable”  $M + 1$  dimensional regret vectors?*
4. We show that with a high probability, the components of the regret vector of UCRL-CMDP can be bounded as  $\tilde{O}\left(S\sqrt{AT^{1.5}}\right)^1$ .
5. We provide a partial characterization of the set of those  $M + 1$ -dimensional regret vectors, which cannot be achieved under any learning algorithm. More specifically, we show that a weighted sum of the  $M + 1$  regrets is necessarily greater than  $O\left(D(p)S\sqrt{AT\log(T)}\right)$ .
6. In many applications, an agent is more sensitive to the cost expenditures of some specific resources as compared to the rest, and a procedure to “tune” the  $M + 1$  dimensional regret vector is essential. We consider the scenario in which the agent can pre-specify the desired bounds on each component of the cost regret vector, and introduce a modification to UCRL-CMDP that allows the agent to keep the cost regrets below these bounds.
7. Regrets of the algorithms proposed in this work scales as  $\tilde{O}(T^{.75})$ . In contrast, the regret of RL algorithms such as UCRL2 of [JOA10] for unconstrained MDPs scales as  $\tilde{O}(T^{.5})$ . This increase is due to the consideration of constraints on costs; and it remains to be seen if this dependency can be reduced to  $\tilde{O}(T^{.5})$ . A more detailed discussion of the key challenges faced during improving this factor, is provided in Section.

<sup>1</sup> $\tilde{O}$  hides factors that are logarithmic in  $T$ .

**Failure of OFU in constrained RL problems:** Consider a two-state  $\mathcal{S} = \{0, 1\}$ , two-action  $\mathcal{A} = \{0, 1\}$  MDP in which the transition probabilities  $p(1, 1, 1) = 1 - \theta$  and  $p(1, 1, 2) = \theta$  are unknown, while remaining probabilities are equal to .5. Assume that  $r(1, a), c(1, a) \equiv 0$  and  $r(2, a), c(2, a) \equiv 1$ , i.e., reward and cost depend only upon the current state. Assume that  $\theta > .5$ , and the average cost threshold satisfies  $c^{ub} < 2\theta/(1 + 2\theta)$ . Since state 2 yields reward at the maximum rate, if  $\theta > .5$  then the optimal control in state 1 is to choose action 1. Thus, if  $\hat{\theta}_t$  and  $\epsilon_t$  denote the estimate of  $\theta$ , and the radius of confidence interval respectively at time  $t$ , then UCRL2 chooses action 1 in state 1 if  $\hat{\theta}_t + \epsilon_t \geq .5$ . Since  $\hat{\theta}_t \rightarrow \theta$  and  $\epsilon_t \rightarrow 0$  as  $T \rightarrow \infty$  [JOA10], we have that when the index of the RL episode is sufficiently large, the agent implements the policy  $\pi(1) = 1, \pi(2) = 1$ . Since the average cost of this policy is  $2\theta/(1 + 2\theta)$ , this means that UCRL2 violates the average cost constraint.

## 2 Preliminaries

Consider a controlled Markov process [Put14]  $s_t, t = 1, 2, \dots, T$ . At each discrete time  $t$ , an agent applies control  $a_t$ . State-space, and action space are denoted by  $\mathcal{S}$  and  $\mathcal{A}$  respectively, and are assumed to be finite. The controlled transition probabilities are denoted  $p := \{p(s, a, s')\}_{s, s' \in \mathcal{S}, a \in \mathcal{A}}$ . Thus,  $p(s, a, s')$  is the probability that system state transitions to state  $s'$  upon applying action  $a$  in state  $s$ . The probabilities  $p(s, a, s')$  are not known to the agent.

The instantaneous reward obtained upon taking an action  $a$  in the state  $s$  is equal to  $r(s, a)$ . Additionally, the agent also incurs  $M$  costs, with the  $i$ -th such cost equal to  $c_i(s, a)$ . Reward and cost functions are denoted by  $r, \{c_i\}_{i=1}^M, \mathcal{S} \times \mathcal{A} \mapsto \mathbb{R}$ , and are known to the agent. Thus, a controlled Markov process in which the agent earns reward and incurs  $M$  costs is defined by the tuple  $\mathcal{CMP} = (\mathcal{S}, \mathcal{A}, p, r, c_1, c_2, \dots, c_M)$ .

A stationary policy  $\pi : \mathcal{S} \mapsto \Delta(\mathcal{A})$ , where  $\Delta(\mathcal{A})$  is the  $|\mathcal{A}|$ -simplex, is a mapping from state  $\mathcal{S}$  to a probability distribution on the action space  $\mathcal{A}$ , and prescribes randomized controls on the basis of the current state  $s_t$ . Thus, under policy  $\pi$ , we have that  $a_t$  is chosen according to the probability distribution  $\pi(s_t)$ .

Consider the controlled Markov process  $s_t$  that starts in state  $s$ , and evolves under the application of a stationary policy  $\pi$ . Let  $\mathbb{E}_\pi(T_{s, s'})$  denote the expected value of the time taken by the process  $s_t$  to hit the state  $s'$ . The MDP  $p$  is communicating if for each pair  $(s, s')$  of states, there is a stationary policy  $\pi$  (which perhaps depends upon the states  $(s, s')$ ), under which  $\mathbb{E}_\pi(T_{s, s'})$  is finite. In this case, the “diameter” of the MDP  $p$  is defined as follows,

$$D(p) := \max_{s, s' \in \mathcal{S}} \left( \min_{\pi} \mathbb{E}_\pi(T_{s, s'}) \right). \quad (1)$$

**Notation:** Throughout, we use boldfont to only denote vectors; for example the vector  $(x_1, x_2, \dots, x_N)$  is denoted by  $\mathbf{x}$ . We use  $\mathbb{N}$  to denote the set of natural numbers,  $\mathbb{R}^M$  to denote the  $M$  dimensional Euclidean space, and  $\mathbb{R}_+^M$  to denote non-negative orthant of  $\mathbb{R}^M$ . For numbers  $x, y \in \mathbb{N}$  that satisfy  $y > x$ , we let  $[x, y] := \{x, x + 1, \dots, y\}$ . Inequalities between two vectors are to be understood componentwise. For an event  $\mathcal{E}$ , we let  $\mathbb{1}(\mathcal{E})$  denote its indicator function. If  $\pi$  is a control policy, then  $\bar{r}(\pi) := \lim_{T \rightarrow \infty} \frac{1}{T} \mathbb{E}_\pi \sum_{t=1}^T r(s_t, a_t)$  denotes its average reward, and similarly  $\bar{c}_i(\pi) := \lim_{T \rightarrow \infty} \frac{1}{T} \mathbb{E}_\pi \sum_{t=1}^T c_i(s_t, a_t)$  denotes its average  $i$ -th cost. For a vector  $x \in \mathbb{R}^N$ , we let  $\|x\|_1$  denote its 1-norm. We let  $\pi_{unif}$  be the policy that in each state  $s$ , chooses each action  $a$  w.p.  $1/|\mathcal{A}|$ . Define the function  $g(t) = t^{25}$ , and let  $\gamma_t \equiv 1/g(T), t \in [1, T]$ .  $\mathbf{0}_M$  denotes the  $M$ -dimensional zero vector consisting of all zeros. For  $x, y \in \mathbb{R}$ , we define  $x \vee y := \max\{x, y\}$ .

### 2.1 Constrained MDPs

We now present some definitions and standard results pertaining to constrained MDPs. These can be found in [Alt99]. We begin with some definitions.

**Definition 1** (Occupation Measure). *Consider the controlled Markov process  $s_t$  evolving under the application of a stationary policy  $\pi$ . Its occupation measure  $\mu_\pi = \{\mu_\pi(s, a) : (s, a) \in \mathcal{S} \times \mathcal{A}\}$  defined as  $\mu_\pi(s, a) := \lim_{T \rightarrow \infty} \frac{1}{T} \mathbb{E}_\pi \sum_{t=1}^T \mathbb{1}(s_t = s, a_t = a)$  describes the average amount of time that the process  $(s_t, a_t)$  spends on each possible state-action pair.*

187 **Definition 2.** Consider a vector  $\mu = \{\mu(s, a)\}_{(s, a) \in \mathcal{S} \times \mathcal{A}}$  that satisfies the constraints (6) and (7)  
 188 below. Define  $SR(\mu)$  to be the following stationary randomized policy. When the state  $s_t$  of the  
 189 environment is equal to  $s$ , the policy chooses the action  $a$  with a probability equal to  $\mu(s, a) /$   
 190  $\sum_{a' \in \mathcal{A}} \mu(s, a')$  if  $\sum_{a' \in \mathcal{A}} \mu(s, a') > 0$ . However, if  $\sum_{a' \in \mathcal{A}} \mu(s, a') = 0$ , then the policy takes an  
 191 action according to some pre-specified rule (e.g. implement  $a_t = 0$ ).

192 **Constrained MDP (CMDP):** Consider the controlled Markov process  $\mathcal{CMP} =$   
 193  $(\mathcal{S}, \mathcal{A}, p, r, c_1, c_2, \dots, c_M)$  in which the instantaneous reward at time  $t$  is given by  $r(s_t, a_t)$ ,  
 194 and the  $i$ -th cost is given by  $c_i(s_t, a_t)$ . The following dynamic optimization problem is a constrained  
 195 Markov Decision Process (CMDP) [Alt99],

$$\max_{\pi} \liminf_{T \rightarrow \infty} \frac{1}{T} \mathbb{E}_{\pi} \sum_{t=1}^T r(s_t, a_t) \quad (2)$$

$$\text{s.t. } \limsup_{T \rightarrow \infty} \frac{1}{T} \mathbb{E}_{\pi} \sum_{t=1}^T c_i(s_t, a_t) \leq c_i^{ub}, i \in [1, M], \quad (3)$$

196 where the maximization above is over the class of all history-dependent policies, and  $c_i^{ub}$  denotes the  
 197 desired upper-bound on the average value of  $i$ -th cost expense.

198 **LP approach for solving CMDPs:** When the controlled transition probabilities  $p(s, a, s')$  are known,  
 199 an optimal policy for the CMDP (2)-(3) can be obtained by solving the following linear program  
 200 (LP),

$$\max_{\mu = \{\mu(s, a) : (s, a) \in \mathcal{S} \times \mathcal{A}\}} \sum_{(s, a) \in \mathcal{S} \times \mathcal{A}} \mu(s, a) r(s, a), \quad (4)$$

$$\text{s.t. } \sum_{(s, a) \in \mathcal{S} \times \mathcal{A}} \mu(s, a) c_i(s, a) \leq c_i^{ub}, i \in [1, M] \quad (5)$$

$$\sum_{a \in \mathcal{A}} \mu(s, a) = \sum_{(s', b) \in \mathcal{S} \times \mathcal{A}} \mu(s', b) p(s', b, s), \quad \forall s \in \mathcal{S}, \quad (6)$$

$$\mu(s, a) \geq 0, \quad \forall (s, a) \in \mathcal{S} \times \mathcal{A}, \quad \sum_{(s, a) \in \mathcal{S} \times \mathcal{A}} \mu(s, a) = 1. \quad (7)$$

201 Let  $\mu^*$  be a solution of the above LP. Then, the stationary randomized policy  $SR(\mu^*)$  solves (2)-(3).  
 202 Moreover it can be shown that its average reward and  $M$  costs are independent of the initial starting  
 203 state  $s_0$ .

## 204 2.2 Learning Algorithms and Regret Vector

205 We will develop reinforcement learning algorithms to solve the finite-time horizon version of the  
 206 CMDP (2)-(3) in case when the probabilities  $p(s, a, s')$  are not known to the agent. Let  $\mathcal{F}_t$  denote  
 207 the sigma-algebra generated by the random variables  $\{(s_{\ell}, a_{\ell})\}_{\ell=1}^{t-1} \cup s_t$ . A learning policy  $\pi$  is a  
 208 collection of maps  $\mathcal{F}_t \mapsto \Delta(\mathcal{A})$ ,  $t = 1, 2, \dots$  that chooses action  $a_t$  on the basis of past operational  
 209 history of the system. In order to measure the performance of a learning algorithm, we define its  
 210 reward and cost regrets.

211 The ‘‘cumulative reward regret’’ until time  $T$ , denoted  $\Delta^{(R)}(T)$ , is defined as,

$$\Delta^{(R)}(T) := r^* T - \sum_{t=1}^T r(s_t, a_t), \quad (8)$$

212 where  $r^*$  is the optimal average reward of the CMDP (2)-(3) when controlled transition probabilities  
 213  $p(s, a, s')$  are known. Note that  $r^*$  is the optimal value of the LP (4)-(7).

214 The ‘‘cumulative cost regret’’ for the  $i$ -th cost until time  $T$  is denoted  $\Delta^{(i)}(T)$ , and is defined as,

$$\Delta^{(i)}(T) := \sum_{t=1}^T c_i(s_t, a_t) - c_i^{ub} T. \quad (9)$$

215 **Remark 1.** In the conventional regret analysis of RL algorithms, the objective is to bound the reward  
 216 regret  $\Delta^{(R)}(T)$ . However, in our setup, due to considerations on the cost expenditures, we also need  
 217 to bound the cost regrets  $\Delta^{(i)}(T)$ . Indeed, as shown in the Section 4, we can force  $\Delta^{(R)}(T)$  to be  
 218 arbitrarily small at the expense of increased cost regrets, and also vice versa.

### 219 3 UCRL-CMDP: A Learning Algorithm for CMDPs

---

#### Algorithm 1 UCRL-CMDP

---

**Input:** State-space  $\mathcal{S}$ , Action-space  $\mathcal{A}$ , Confidence parameter  $\delta$ , Time horizon  $T$

**Initialize:** Set  $t := 1$ , and observe the initial state  $s_1$ .

**for** Episodes  $k = 1, 2, \dots$  **do**

**Initialize Episode  $k$ :**

1. Set the start time of episode  $k$ ,  $\tau_k := t$ . For all state-action tuples  $(s, a) \in \mathcal{S} \times \mathcal{A}$ , initialize the number of visits within episode  $k$ ,  $n_k(s, a) = 0$ .
2. For all  $(s, a) \in \mathcal{S} \times \mathcal{A}$  set  $N_{\tau_k}(s, a)$ , i.e., the number of visits to  $(s, a)$  prior to episode  $k$ . Also set the transition counts  $N_{\tau_k}(s, a, s')$  for all  $(s, a, s') \in \mathcal{S} \times \mathcal{A} \times \mathcal{S}$ .
3. Compute the empirical estimate  $\hat{p}_t$  of the MDP as in (10).

**Compute Policy  $\tilde{\pi}_k$ :**

1. Let  $\mathcal{C}_{\tau_k}$  be the set of plausible MDPs as in (12).
2. Solve (14)-(17) to obtain  $\tilde{\pi}_k$ .
3. In case (14)-(17) is infeasible, choose  $\tilde{\pi}_k$  to be some pre-determined policy (chosen at time  $t = 0$ ).

**Implement  $\tilde{\pi}_k$ :**

**while**  $n_k(s_t, a_t) < N_k(s_t, a_t)$  **do**

1. Sample  $a_t$  according to the distribution  $\tilde{\pi}_k(\cdot | s_t)$ . Observe reward  $r(s_t, a_t)$ , and observe next state  $s_{t+1}$ .
2. Update  $n_k(s_t, a_t) = n_k(s_t, a_t) + 1$ .
3. Set  $t := t + 1$ .

**end while**

**end for**

---

220 The proposed algorithm, Algorithm 1, maintains empirical estimates of the unknown transition  
 221 probabilities as follows,

$$\hat{p}_t(s, a, s') = \frac{N_t(s, a, s')}{N_t(s, a) \vee 1}, \forall s, s' \in \mathcal{S}, a \in \mathcal{A}, \quad (10)$$

222 where

$$N_t(s, a) = \sum_{l < t} \mathbb{1}\{s_l = s, a_l = a\}, N_t(s, a, s') = \sum_{l < t-1} \mathbb{1}\{s_l = s, a_l = a, s_{l+1} = s'\}. \quad (11)$$

223 **Confidence Intervals:** Additionally, it also maintains confidence interval  $\mathcal{C}_t$  associated with the  
 224 estimate  $\hat{p}_t$  as follows,

$$\mathcal{C}_t := \{p' = \{p(s, a, s')\}_{s, s' \in \mathcal{S}, a \in \mathcal{A}} : \|p'(s, a, \cdot) - \hat{p}_t(s, a, \cdot)\|_1 \leq \epsilon_t(s, a), \forall (s, a)\}, \quad (12)$$

225 where

$$\epsilon_t(s, a) := \sqrt{\frac{14|\mathcal{S}| \log(2|\mathcal{A}|t/\delta)}{N_t(s, a) \vee 1}}. \quad (13)$$

226 **Episode:** Algorithm 1 proceeds in episodes, and utilizes a single stationary control policy within an  
 227 episode. A new episode begins each time the number of visits to some state-action pair  $(s, a)$  doubles.  
 228 Let  $\tau_k$  denote the start time of episode  $k$ .  $k$ -th episode is denoted by  $\mathcal{E}_k := [\tau_k, \tau_{k+1} - 1]$ , and it  
 229 comprises of  $|\tau_{k+1} - \tau_k|$  consecutive time-steps.

At the beginning of  $\mathcal{E}_k$ , the agent solves the following *constrained* optimization problem in which the decision variables are (i) Occupation measure  $\mu = \{\mu(s, a) : (s, a) \in \mathcal{S} \times \mathcal{A}\}$  of the controlled process, and (ii) “Candidate” MDP  $p'$ ,

$$\max_{\mu, p'} \sum_{(s, a) \in \mathcal{S} \times \mathcal{A}} \mu(s, a) r(s, a), \quad (14)$$

$$\text{s.t.} \quad \sum_{(s, a) \in \mathcal{S} \times \mathcal{A}} \mu(s, a) c_i(s, a) \leq c_i^{ub}, i \in [1, M] \quad (15)$$

$$\sum_{a \in \mathcal{A}} \mu(s, a) = \sum_{(s', b) \in \mathcal{S} \times \mathcal{A}} \mu(s', b) p'(s', b, s), \quad \forall s \in \mathcal{S}, \quad (16)$$

$$\mu(s, a) \geq 0 \quad \forall (s, a), \sum_{(s, a)} \mu(s, a) = 1, \quad p' \in \mathcal{C}_{\tau_k}. \quad (17)$$

The maximization w.r.t.  $p'$  denotes that the agent is optimistic regarding the belief of the “true” (but unknown) MDP  $p$ , while that w.r.t.  $\mu$  ensures that agent optimizes its control strategy for this optimistic MDP. The constraints (15) ensure that the cost expenditures do not exceed the thresholds  $\{c_i^{ub}\}_{i=1}^M$ . In case the problem (14)-(17) is feasible, let  $(\tilde{\mu}_k, \tilde{p}_k)$  denote a solution. Within the episode  $\mathcal{E}_k$ , at each time  $t$ , the agent chooses  $a_t$  according to  $SR(\tilde{\mu}_k)$  w.p.  $1 - \gamma_t$ . With a probability  $\gamma_t$ , it chooses  $a_t$  uniformly at random from the set  $\mathcal{A}$ . However, in the event the LP (14)-(17) is infeasible, the agent implements an arbitrary stationary control policy that has been chosen at time  $t = 0$ . This stationary policy implemented within  $\mathcal{E}_k$  is denoted by  $\tilde{\pi}_k$ .

We make the following assumptions on the MDP  $p$  while analyzing UCRL-CMDP.

- Assumption 1.** (i) The MDP  $p = \{p(s, a, s')\}_{s, s' \in \mathcal{S}, a \in \mathcal{A}}$  is communicating.  
(ii) The CMDP (2)-(3) is feasible, i.e., there exists a policy under which the average cost constraints (3) are satisfied.  
(iii) Without loss of generality, we assume that the magnitude of rewards and costs are upper-bounded by 1, i.e.,

$$|r(\cdot, \cdot)|, |c_i(\cdot, \cdot)| < 1.$$

Hence, if  $r^*$  denotes optimal reward rate of (2)-(3), then  $r^* < 1$ . Moreover, the cost bounds  $\{c_i^{ub}\}_{i=1}^M$  can be taken to be less than 1.

We establish the following bound on the regrets of UCRL-CMDP. Its proof is deferred to the Appendix.

**Theorem 1.** Suppose that UCRL-CMDP, i.e., Algorithm 1 is run for  $T$  time steps on an MDP  $p$  that satisfies Assumption 1. Then, with probability at least  $1 - \delta$ , the reward regret  $\Delta^{(R)}(T)$  and cost regrets  $\Delta^{(i)}(T), i \in [1, M]$  are upper-bounded as follows,

$$\Delta^{(R)}(T) \leq 34 \cdot S \sqrt{AT^{1.5} \log(T/\delta)}, \quad \Delta^{(i)}(T) \leq 34 \cdot S \sqrt{AT^{1.5} \log(T/\delta)}, \quad \forall i \in [1, M]. \quad (18)$$

Letting  $\delta = 1/T$  in the above, we obtain that

$$\mathbb{E} \Delta^{(R)}(T) \leq 34 \cdot S \sqrt{2AT^{1.5} \log(T)}, \quad \Delta^{(i)}(T) \leq 34 \cdot S \sqrt{2AT^{1.5} \log(T)}, \quad \forall i \in [1, M]. \quad (19)$$

## 4 Learning Under Bounds on Cost Regret

Under UCRL-CMDP, the upper-bounds derived in Theorem 1 are the same for reward and  $M$  cost regrets. However, in many practical applications, an agent is more sensitive to over-utilizing certain specific costs, as compared to the other costs. Thus, in this section, we derive algorithms which enable the agent to tune the upper-bounds on the regrets of different costs.

Let  $\mathbf{b} = (b_1, b_2, \dots, b_M) \in \mathbb{R}_+^M$  be a vector chosen by the agent that desires the cost regrets  $\Delta^{(i)}(T)$  (9) to be bounded as follows

$$\mathbb{E} \Delta^{(i)}(T) \leq b_i \sqrt{T^{1.5} \log(T/\delta)}, \quad \forall i \in [1, M]. \quad (20)$$

We now derive learning algorithm which maximizes the cumulative reward while ensuring that the constraints (20) on the cost regret vector are satisfied. We also bound its reward regret  $\Delta^{(R)}(T)$ .

264 **Assumption 2.** *There exists a stationary policy under which the average costs are strictly below the*  
 265 *thresholds  $c_i^{ub}$ . More precisely, there exists an  $\epsilon > 0$ , and a stationary policy  $\pi_{feas.}$ , such that we*  
 266 *have  $\bar{c}_i(\pi_{feas.}) < c_i^{ub} - \epsilon, \forall i \in [1, M]$ . Define*

$$\eta := \min_{i \in [1, M]} \{c_i^{ub} - \epsilon - \bar{c}_i(\pi_{feas.})\}. \quad (21)$$

267 **Modified UCRL-CMDP:** The modified algorithm maintains empirical estimates  $\hat{p}_t$  using (10), and  
 268 confidence intervals  $\mathcal{C}_t$  as in (12) in exactly the same manner as UCRL-CMDP (Algorithm 1) does. It  
 269 also proceeds in episodes, and uses a single stationary control policy within an episode. However, at  
 270 the beginning of each episode  $k$ , it solves the following optimization problem, that is a modification  
 271 of the problem (14)-(17) that is solved by UCRL-CMDP. More concretely, the cost constraints (15)  
 272 are replaced by the following constraints on costs

$$\text{s.t.} \quad \sum_{(s,a) \in \mathcal{S} \times \mathcal{A}} \mu(s,a) c_i(s,a) \leq c_i^{ub} - d_i, \quad i \in [1, M] \quad (22)$$

273 where  $d_i := (34 - b_i) / T \cdot S \sqrt{A T^{1.5} \log(T/\delta)}$ ,  $i \in [1, M]$ . The stationary policy  $\tilde{\pi}_k$  implemented  
 274 within  $\mathcal{E}_k$  is obtained from the solution of the modified optimization problem in exactly the same  
 275 manner as UCRL-CMDP.

276 **Theorem 2.** *Suppose that the modified UCRL-CMDP is run for  $T$  time steps on an MDP  $p$  that*  
 277 *satisfies Assumption 1 and Assumption 2. Then, with a probability at least  $1 - \delta$ , the reward regret*  
 278  *$\Delta^{(R)}(T)$  and cost regrets  $\Delta^{(i)}(T)$ ,  $i \in [1, M]$  are upper-bounded as follows,*

$$\Delta^{(R)}(T) \leq \left(34 + \left(34 - \min_i b_i\right) \cdot (\hat{\eta}/\eta)\right) \cdot S \sqrt{A T^{1.5} \log(T/\delta)}, \quad (23)$$

$$\Delta^{(i)}(T) \leq b_i \cdot S \sqrt{A T^{1.5} \log(T/\delta)}, \quad \forall i \in [1, M]. \quad (24)$$

#### 279 4.1 Achievable Regret Vectors

280 Let  $\lambda = \{\lambda_i\}_{i=1}^M$  be a vector satisfying  $\lambda \geq \mathbf{0}_M$ . Consider the Lagrangian relaxation of (2)-(3),

$$\mathcal{L}(\lambda; \pi) := \liminf_{T \rightarrow \infty} \frac{1}{T} \mathbb{E}_\pi \sum_{t=1}^T \left\{ r(s_t, a_t) + \sum_{i=1}^M \lambda_i (c_i^{ub} - c_i(s_t, a_t)) \right\}. \quad (25)$$

281 Consider its associated dual function [Ber97],  $\mathcal{D}(\lambda) := \max_\pi \mathcal{L}(\lambda; \pi)$ , and the dual problem

$$\min_{\lambda \geq \mathbf{0}} \mathcal{D}(\lambda). \quad (26)$$

282 Recall that for the CMDP (2)-(3), a problem instance is specified by the controlled Markov process  
 283  $\mathcal{CMP} = (\mathcal{S}, \mathcal{A}, p, r, c_1, c_2, \dots, c_M)$ , and the cost bounds  $c_i^{ub}, i \in [1, M]$ . The following result is  
 284 proved in the appendix.

285 **Theorem 3.** *Consider a learning algorithm  $\phi$ . Then, there is a problem instance  $\mathcal{CMP}$  such that the*  
 286 *regrets  $\Delta^{(R)}(T)$ ,  $\{\Delta^{(i)}(T)\}_{i=1}^M$  under  $\phi$  satisfy*

$$\mathbb{E}_\phi \Delta^{(R)}(T) + \sum_{i=1}^M \lambda_i^* \mathbb{E}_\phi \Delta^{(i)}(T) \geq .015 \cdot \sqrt{D(p)SA}, \quad (27)$$

287 where  $\lambda^*$  is an optimal solution of the dual problem (26).

## 288 5 Conclusions and Future Work

289 In this work, we initiate a study to develop learning algorithms that simultaneously control all the  
 290 components of the regret vector while controlling unknown MDPs. We note that the regret bounds  
 291 of our algorithms are  $\tilde{O}(T^{.75})$ , which is larger than the  $\tilde{O}(T^{.5})$  dependence for unconstrained RL  
 292 problems. The key challenge involved in reducing this dependence, is the requirement to *tightly*  
 293 control all the  $M+1$  components of the regret vector *simultaneously*. An interesting research problem  
 294 is to characterize the set of achievable regret vectors. Another interesting question is whether it is  
 295 possible to bound the norm of the regret vector as  $\tilde{O}(T^{.5})$ , so as to recover the regret growth-rate of  
 296 unconstrained RL problems.



## Broader Impact

The work in this paper studies the problem of controlling unknown MDPs under constraints on cost expenditures. The work in this paper is general enough that there is no particular application foreseen. This work does not present any foreseeable societal consequence.

## References

- [Alt99] Eitan Altman. *Constrained Markov Decision Processes*. Chapman and Hall/CRC, March 1999.
- [AO07] Peter Auer and Ronald Ortner. Logarithmic online regret bounds for undiscounted reinforcement learning. In *Advances in Neural Information Processing Systems*, pages 49–56, 2007.
- [AS91] Eitan Altman and Adam Schwartz. Adaptive control of constrained Markov chains. *IEEE Transactions on Automatic Control*, 36(4):454–462, 1991.
- [Ber97] Dimitri P Bertsekas. *Nonlinear programming*, volume 48. Taylor & Francis, 1997.
- [BKS13] A. Badanidiyuru, R. Kleinberg, and A. Slivkins. Bandits with knapsacks. In *2013 IEEE 54th Annual Symposium on Foundations of Computer Science*, pages 207–216, Oct 2013.
- [BKS18] Ashwinkumar Badanidiyuru, Robert Kleinberg, and Aleksandrs Slivkins. Bandits with knapsacks. *J. ACM*, 65(3):13:1–13:55, 2018.
- [Bor97] Vivek S Borkar. Stochastic approximation with two time scales. *Systems & Control Letters*, 29(5):291–294, 1997.
- [Bor05] Vivek S Borkar. An actor-critic algorithm for constrained markov decision processes. *Systems & control letters*, 54(3):207–213, 2005.
- [BT02] Ronen I Brafman and Moshe Tennenholtz. R-max-a general polynomial time algorithm for near-optimal reinforcement learning. *Journal of Machine Learning Research*, 3(Oct):213–231, 2002.
- [BT09] Peter L. Bartlett and Ambuj Tewari. REGAL: A regularization based algorithm for reinforcement learning in weakly communicating mdps. In *Proceedings of the Twenty-Fifth Conference on Uncertainty in Artificial Intelligence, Montreal, QC, Canada, June 18-21, 2009*, pages 35–42. AUAI Press, 2009.
- [BV04] Stephen Boyd and Lieven Vandenbergh. *Convex optimization*. Cambridge university press, 2004.
- [CJS15] Richard Combes, Chong Jiang, and Rayadurgam Srikant. Bandits with budgets: Regret lower bounds and optimal algorithms. In *Proceedings of the 2015 ACM SIGMETRICS International Conference on Measurement and Modeling of Computer Systems, Portland, OR, USA, June 15-19, 2015*, pages 245–257, 2015.
- [DQZL13] Wenkui Ding, Tao Qin, Xu-Dong Zhang, and Tie-Yan Liu. Multi-armed bandit with budget constraint and variable costs. In *Proceedings of the Twenty-Seventh AAAI Conference on Artificial Intelligence, July 14-18, 2013, Bellevue, Washington, USA.*, 2013.
- [HLGHLM03] Onésimo Hernández-Lerma, Juan González-Hernández, and Raquiel R López-Martínez. Constrained average cost markov control processes in borel spaces. *SIAM Journal on Control and Optimization*, 42(2):442–468, 2003.
- [HLL98] Onésimo Hernández-Lerma and Jean B Lasserre. Approximation schemes for infinite linear programs. *SIAM Journal on Optimization*, 8(4):973–988, 1998.
- [JOA10] Thomas Jaksch, Ronald Ortner, and Peter Auer. Near-optimal regret bounds for reinforcement learning. *Journal of Machine Learning Research*, 11(Apr):1563–1600, 2010.
- [Pau68] Paul J. Schweitzer. Perturbation theory and finite markov chains. *Journal of Applied Probability*, 5(2):401–413, 1968.

- [Put14] Martin L. Puterman. *Markov Decision Processes.: Discrete Stochastic Dynamic Programming*. John Wiley & Sons, 2014.
- [S. 12] S. P. Meyn, and R. L. Tweedie. *Markov chains and Stochastic Stability*. Springer Science & Business Media, 2012.
- [SB98] Richard S. Sutton and Andrew G. Barto. *Reinforcement learning - an introduction*. Adaptive computation and machine learning. MIT Press, 1998.
- [Sen09] Linn I. Sennott. *Stochastic dynamic programming and the control of queueing systems*, volume 504. John Wiley & Sons, 2009.
- [Tor02] Torgny Lindvall. *Lectures on the coupling method*. Courier Corporation, 2002.

## Supplementary Material

### A Proof of Theorem 1

The proof follows closely the proof of Theorem 2 of [JOA10] with some subtle differences.

*Regret Decomposition* : Let  $K$  denote the total number of episodes incurred until  $T$ . Let  $n_k(s, a)$  be the number of visits to  $(s, a)$  during episode  $k$ , i.e.,

$$n_k(s, a) := \sum_{t \in \mathcal{E}_k} \mathbb{1}\{s_t = s, a_t = a\}, s \in \mathcal{S}, a \in \mathcal{A}. \quad (28)$$

Consider the regrets incurred during  $k$ -th episode, i.e., let,

$$\Delta_k^{(R)} := \sum_{(s,a) \in \mathcal{S} \times \mathcal{A}} n_k(s, a) (r^* - r(s, a)), \quad (29)$$

$$\Delta_k^{(i)} := \sum_{(s,a) \in \mathcal{S} \times \mathcal{A}} n_k(s, a) (c_i(s, a) - c_i^{ub}), i \in [1, M]. \quad (30)$$

The cumulative regrets  $\Delta^{(R)}(T), \{\Delta^{(i)}(T)\}_{i=1}^M$  can be decomposed into the sum of “episodic regrets” as follows,

$$\Delta^{(R)}(T) = \sum_{k=1}^K \Delta_k^{(R)}, \quad (31)$$

$$\Delta^{(i)}(T) = \sum_{k=1}^K \Delta_k^{(i)}, i \in [1, M]. \quad (32)$$

We further decompose the episodic regrets as follows,

$$\Delta_k^{(R)} = \Delta_k^{(R)} \mathbb{1}\{p \notin \mathcal{C}_{\tau_k}\} + \Delta_k^{(R)} \mathbb{1}\{p \in \mathcal{C}_{\tau_k}\}, \quad (33)$$

and similarly for  $\{\Delta_k^{(i)}\}_{i=1}^M$ . Thus, the cumulative regret  $\Delta^{(R)}(T)$  in (31) can be written as follows,

$$\Delta^{(R)}(T) = \sum_{k=1}^K \Delta_k^{(R)} \mathbb{1}\{p \notin \mathcal{C}_{\tau_k}\} + \sum_{k=1}^K \Delta_k^{(R)} \mathbb{1}\{p \in \mathcal{C}_{\tau_k}\}, \quad (34)$$

and similarly for the  $M$  cost regrets. The two summations in the above expression are now bounded separately.

#### A.1 Regret When Confidence Intervals Fail ( $p \notin \mathcal{C}_{\tau_k}$ )

We can upper-bound the first summation in (34) as follows.

**Lemma 1.** *We have that with a probability at least  $1 - \frac{\delta}{12T^{5/4}}$ ,*

$$\sum_{k=1}^K \Delta_k^{(R)} \mathbb{1}\{p \notin \mathcal{C}_{\tau_k}\} \leq \sqrt{T}, \text{ and also },$$

$$\sum_{k=1}^K \Delta_k^{(i)} \mathbb{1}\{p \notin \mathcal{C}_{\tau_k}\} \leq \sqrt{T}, \forall i \in [1, M].$$

370 *Proof.* The proof is similar to the discussion in Section 4.2 of [JOA10]; the difference being that we  
 371 need to upper-bound multiple  $(M + 1)$  regrets simultaneously. The proof carries over to our set-up  
 372 since the following inequalities hold true,

$$\begin{aligned} \sum_{k=1}^K \Delta_k^{(R)} \mathbb{1} \{p \notin \mathcal{C}_{\tau_k}\} &\leq \sqrt{T} + \sum_{t=T^{1/4}}^T t \mathbb{1} \{p \notin \mathcal{C}_t\}, \\ \sum_{k=1}^K \Delta_k^{(R)} \mathbb{1} \{p \notin \mathcal{C}_{\tau_k}\} &\leq \sqrt{T} + \sum_{t=T^{1/4}}^T t \mathbb{1} \{p \notin \mathcal{C}_t\}, \forall i \in [1, M]. \end{aligned}$$

373 The statement then follows by observing that  $\mathbb{P}(\exists t : T^{1/4} < t < T : p \notin \mathcal{C}_t) < \frac{\delta}{12T^{5/4}}$ .  $\square$

## 374 A.2 Regret When Confidence Intervals are True ( $p \in \mathcal{C}_{\tau_k}$ )

375 This section derives upper-bounds on the second term in the expression on the r.h.s. of (34). In  
 376 the event  $\{p \in \mathcal{C}_{\tau_k}\}$ , the problem (14)-(17) that needs to be solved by the agent is feasible. This is  
 377 seen to be true since the true MDP parameters  $p(s, a, s')$  satisfy the constraints (17), and moreover,  
 378 the CMDP (2)-(3) with controlled transition probabilities set equal to the true MDP  $p$  is feasible  
 379 (Assumption 1). Denote by  $r_k^*, c_{i,k}^*$  the reward and costs associated with a solution to (14)-(17). Since  
 380  $p \in \mathcal{C}_{\tau_k}$ , we have,

$$r_k^* \geq r^*, \quad (35)$$

381 and also,

$$c_{i,k}^* \leq c_i^{ub}, \quad i \in [1, M]. \quad (36)$$

382 In case  $p \in \mathcal{C}_{\tau_k}$ , the problem (14)-(17) is feasible, so that  $\tilde{\pi}_k$  is described as follows: w.p.  $1 - \gamma_t$ ,  
 383 choose  $a_t$  according to  $SR(\tilde{\mu}_k)$ , while with a probability  $\gamma_t$ , choose action  $a_t$  uniformly at random  
 384 from the action-space  $\mathcal{A}$ . It then follows by performing a sensitivity analysis of Markov chain, i.e.,  
 385 Lemma 10, that the average rewards and costs of  $\tilde{\pi}_k$  satisfy the following relations,

$$\bar{r}(\tilde{\pi}_k) \geq \bar{r}(SR(\tilde{\mu}_k)) - O(\gamma_t) = r_k^* - O(\gamma_{\tau_k}), \quad (37)$$

$$\text{and } \bar{c}_i(\tilde{\pi}_k) \leq \bar{c}_i(SR(\tilde{\mu}_k)) + O(\gamma_{\tau_k}) = c_{i,k}^* + O(\gamma_{\tau_k}). \quad (38)$$

386 Substituting these two inequalities into (29) and (30), we obtain the following,

$$\Delta_k^{(R)} \mathbb{1} \{p \in \mathcal{C}_{\tau_k}\} \leq \sum_{(s,a) \in \mathcal{S} \times \mathcal{A}} n_k(s, a) (r_k^* - r(s, a)) + \sum_{(s,a)} n_k(s, a) O(\gamma_{\tau_k}), \quad (39)$$

$$\Delta_k^{(i)} \mathbb{1} \{p \in \mathcal{C}_{\tau_k}\} \leq \sum_{(s,a)} n_k(s, a) (c_i(s, a) - c_{i,k}^*) + \sum_{(s,a)} n_k(s, a) O(\gamma_{\tau_k}), i \in [1, M]. \quad (40)$$

387 Utilizing the result of Lemma 12, the inequalities (39) and (40) can be written as follows,

$$\begin{aligned} &\Delta_k^{(R)} \mathbb{1} \{p \in \mathcal{C}_{\tau_k}\} \\ &\leq \sum_{(s,a) \in \mathcal{S} \times \mathcal{A}} n_k(s, a) \left( \sum_{s' \in \mathcal{S}} \tilde{p}_k(s, a, s') \left( \sum_{b \in \mathcal{A}} [SR(\tilde{\mu}_k)](b|s') v_k^{(R)}(s', b) \right) - v_k^{(R)}(s, a) \right) \\ &+ \sum_{(s,a) \in \mathcal{S} \times \mathcal{A}} n_k(s, a) O(\gamma_{\tau_k}), \end{aligned} \quad (41)$$

388

$$\begin{aligned} &\Delta_k^{(i)} \mathbb{1} \{p \in \mathcal{C}_{\tau_k}\} \\ &\leq \sum_{(s,a) \in \mathcal{S} \times \mathcal{A}} n_k(s, a) \left( v_k^{(i)}(s, a) - \sum_{s' \in \mathcal{S}} \tilde{p}_k(s, a, s') \left( \sum_{b \in \mathcal{A}} [SR(\tilde{\mu}_k)](b|s') v_k^{(i)}(s', b) \right) \right) \\ &+ \sum_{(s,a) \in \mathcal{S} \times \mathcal{A}} n_k(s, a) O(\gamma_{\tau_k}), \forall i \in [1, M], \end{aligned} \quad (42)$$

where  $v^{(R)}, v^{(i)} : \mathcal{S} \times \mathcal{A} \mapsto \mathbb{R}$  can be interpreted as the differential “reward/cost-to-go functions” associated with the policy  $SR(\tilde{\mu}_k)$  that is optimal for (14)-(17). The above inequalities can be written as follows

$$\Delta_k^{(R)} \mathbb{1} \{p \in \mathcal{C}_{\tau_k}\} \leq \Delta_{k,1}^{(R)} + \Delta_{k,2}^{(R)} + \Delta_{k,3}^{(R)}, \quad (43)$$

where

$$\begin{aligned} \Delta_{k,1}^{(R)} &:= \sum_{(s,a) \in \mathcal{S} \times \mathcal{A}} n_k(s,a) \left( \sum_{s' \in \mathcal{S}} [\tilde{p}_k(s,a,s') - p(s,a,s')] \left( \sum_{b \in \mathcal{A}} [SR(\tilde{\mu}_k)](b|s') v_k^{(R)}(s',b) \right) \right), \\ \Delta_{k,2}^{(R)} &:= \sum_{(s,a) \in \mathcal{S} \times \mathcal{A}} n_k(s,a) \left( \sum_{s'} p(s,a,s') \left( \sum_b [SR(\tilde{\mu}_k)](b|s') v_k^{(R)}(s',b) \right) - v_k^{(R)}(s,a) \right), \\ \Delta_{k,3}^{(R)} &:= \sum_{(s,a) \in \mathcal{S} \times \mathcal{A}} n_k(s,a) O(\gamma_{\tau_k}). \end{aligned}$$

Similarly,

$$\Delta_k^{(i)} \mathbb{1} \{p \in \mathcal{C}_{\tau_k}\} \leq \Delta_{k,1}^{(i)} + \Delta_{k,2}^{(i)} + \Delta_{k,3}^{(i)}, \quad (44)$$

where,

$$\begin{aligned} \Delta_{k,1}^{(i)} &:= \sum_{(s,a) \in \mathcal{S} \times \mathcal{A}} n_k(s,a) \left( \sum_{s' \in \mathcal{S}} [\tilde{p}_k(s,a,s') - p(s,a,s')] \left( \sum_{b \in \mathcal{A}} [SR(\tilde{\mu}_k)](b|s') v_k^{(i)}(s',b) \right) \right) \\ \Delta_{k,2}^{(i)} &:= \sum_{(s,a) \in \mathcal{S} \times \mathcal{A}} n_k(s,a) \left( \sum_{s' \in \mathcal{S}} p(s,a,s') \left( \sum_{b \in \mathcal{A}} [SR(\tilde{\mu}_k)](b|s') v_k^{(i)}(s',b) \right) - v_k^{(i)}(s,a) \right), \\ \Delta_{k,3}^{(i)} &:= \sum_{(s,a) \in \mathcal{S} \times \mathcal{A}} n_k(s,a) O(\gamma_{\tau_k}), \quad i \in [1, M]. \end{aligned}$$

We now bound the terms  $\Delta_{k,1}^{(R)}, \Delta_{k,1}^{(i)}$  and  $\Delta_{k,2}^{(R)}, \Delta_{k,2}^{(i)}$ , and  $\Delta_{k,3}^{(R)}, \Delta_{k,3}^{(i)}$  separately.

**Bounding  $\Delta_{k,1}^{(R)}, \Delta_{k,1}^{(i)}$ :**

**Lemma 2.**

$$\begin{aligned} \sum_{k=1}^K \Delta_{k,1}^{(R)} &\leq O(g(T)) (\sqrt{2} + 1) \sqrt{SAT \log \left( \frac{T}{\delta} \right)}, \text{ and similarly} \\ \sum_{k=1}^K \Delta_{k,1}^{(i)} &\leq O(g(T)) (\sqrt{2} + 1) \sqrt{SAT \log \left( \frac{T}{\delta} \right)}, \forall i \in [1, M]. \end{aligned} \quad (45)$$

*Proof.* It follows from Lemma 12 that  $|v_k^{(R)}|, |v_k^{(i)}|$  are upper-bounded as  $O(1/\gamma_t) = O(g(T))$ . We thus have the following,

$$\Delta_{k,1}^{(R)} = \sum_{(s,a) \in \mathcal{S} \times \mathcal{A}} n_k(s,a) \left( \sum_{s' \in \mathcal{S}} [\tilde{p}_k(s,a,s') - p(s,a,s')] \left( \sum_{b \in \mathcal{A}} \tilde{\pi}_k(b|s') v_k^{(R)}(s',b) \right) \right) \quad (46)$$

$$\leq \sum_{(s,a) \in \mathcal{S} \times \mathcal{A}} n_k(s,a) \|\tilde{p}_k(s,a,\cdot) - p(s,a,\cdot)\|_1 O(g(T))$$

$$\leq O(g(T)) \sum_{(s,a)} n_k(s,a) \epsilon_{\tau_k}(s,a)$$

$$= O(g(T)) \sum_{(s,a) \in \mathcal{S} \times \mathcal{A}} n_k(s,a) \sqrt{\frac{\alpha \log(\tau_k/\delta)}{N_{\tau_k}(s,a)}}, \quad (47)$$

where the first inequality follows from Lemma 12, and the second from UCB confidence interval (12), (13). Similarly we obtain,

$$\Delta_{k,1}^{(i)} \leq O(g(T)) \sum_{(s,a) \in \mathcal{S} \times \mathcal{A}} n_k(s,a) \sqrt{\frac{\alpha \log(\tau_k/\delta)}{N_{\tau_k}(s,a)}}. \quad (48)$$

The proof is completed by summing up the inequalities (47) and (48) over episodes  $k$ .  $\square$

**Bounding  $\Delta_{k,2}^{(R)}, \Delta_{k,2}^{(i)}$ :**

**Lemma 3.** *We have,*

$$\mathbb{P} \left( \sum_{k=1}^K \Delta_{k,2}^{(R)} \leq x; \sum_{k=1}^K \Delta_{k,2}^{(i)} \leq x \forall i \in [1, M] \right) \geq 1 - \frac{(M+1)\delta}{12T^{5/4}}, \quad (49)$$

where  $x = O(g(T)) \sqrt{2T \cdot \frac{5}{4} \log \left( \frac{8T(M+1)}{\delta} \right)} + O(g(T)) S A \log \left( \frac{8T}{SA} \right)$ .

*Proof.* Let  $k_t$  denote the index of the ongoing episode at time  $t$ , i.e.,

$$k_t := \max \{k : \tau_k \leq t\}.$$

Consider the following martingale difference sequences  $m_t^{(R)}, \{m_t^{(i)}\}_{i=1}^M$ ,

$$m_t^{(R)} := \mathbb{1} \{p \in \mathcal{C}_{\tau_{k_t}}\} \left( v_{k_t}^{(R)}(s_{t+1}, a_{t+1}) - \sum_{(s',b)} p(s_t, a_t, s') \tilde{\pi}_{k_t}(b|s') v_{k_t}^{(R)}(s', b) \right)$$

$$m_t^{(i)} := \mathbb{1} \{p \in \mathcal{C}_{\tau_{k_t}}\} \left( v_{k_t}^{(i)}(s_{t+1}, a_{t+1}) - \sum_{(s',b)} p(s_t, a_t, s') \tilde{\pi}_{k_t}(b|s') v_{k_t}^{(i)}(s', b) \right), i \in [1, M].$$

We have

$$\begin{aligned} \Delta_{k,2}^{(R)} &= \sum_{t=\tau_k}^{\tau_{k+1}-1} m_t^{(R)} + v_k^{(R)}(s_{\tau_{k+1}}, a_{\tau_{k+1}}) - v_k^{(R)}(s_{\tau_k}, a_{\tau_k}) \\ &\leq \sum_{t=\tau_k}^{\tau_{k+1}-1} m_t^{(R)} + O(g(T)), i \in [1, M], \end{aligned} \quad (50)$$

where, the inequality follows from Lemma 12. Summing the above over episodes  $k$ , we obtain

$$\sum_{k=1}^K \Delta_{k,2}^{(R)} \leq \sum_{t=1}^T m_t^{(R)} + K O(g(T)), \text{ and similarly} \quad (51)$$

$$\sum_{k=1}^K \Delta_{k,2}^{(i)} \leq \sum_{t=1}^T m_t^{(i)} + K O(g(T)), \quad (52)$$

where  $K$  is the total number of episodes until time  $T$ . Since it follows from Lemma 12 that  $|m_t^{(R)}|, |m_t^{(i)}| \leq 2 O(g(T))$ . If  $\epsilon > 0$ , then it follows from Azuma-Hoeffding inequality that  $\mathbb{P} \left( \sum_{t=1}^T m_t^{(R)} \geq \epsilon \right) \leq \exp \left( -\frac{\epsilon^2}{2T O(g(T))^2} \right)$ , and similarly for  $\sum_{t=1}^T m_t^{(i)}$ . We then use union bound in order to obtain

$$\mathbb{P} \left( \sum_{t=1}^T m_t^{(R)} < \epsilon; \sum_{t=1}^T m_t^{(i)} < \epsilon, \forall i \in [1, M] \right) \geq 1 - (M+1) \exp \left( -\frac{\epsilon^2}{2T O(g(T))^2} \right).$$

By letting  $\epsilon = O(g(T)) \sqrt{2T \cdot \frac{5}{4} \log \left( \frac{8T(M+1)}{\delta} \right)}$ , we deduce that on a set that has a probability larger than  $1 - \frac{\delta}{12T^{5/4}}$ , the quantities  $\sum_{t=1}^T m_t^{(R)}, \left\{ \sum_{t=1}^T m_t^{(i)} : i \in [1, M] \right\}$  are upper-bounded by

$$O(g(T)) \sqrt{2T \cdot \frac{5}{4} \log \left( \frac{8T(M+1)}{\delta} \right)}.$$

416 The quantity  $K$ , i.e. the total number of episodes incurred during  $T$  steps, can be upper-bounded  
 417 similar to [JOA10] Appendix C.2 as follows,

$$K \leq S A \log \left( \frac{8T}{SA} \right). \quad (53)$$

418 Proof is completed by combining (51), (52), (53) with the probabilistic bounds on  
 419  $\sum_{t=1}^T m_t^{(R)}, \left\{ \sum_{t=1}^T m_t^{(i)} \right\}_{i \in [1, M]}$ ,  $K$  discussed above.  $\square$

420 **Bounding  $\Delta_{k,3}^{(R)}, \Delta_{k,3}^{(i)}$ .**

421 **Lemma 4.** *We have,*

$$\sum_k \Delta_{k,3}^{(R)} = \sum_k \frac{\sum_{(s,a)} n_k(s,a)}{g(T)} = \frac{T}{g(T)}.$$

422 **Bounding  $\Delta_k^{(R)} \mathbb{1}\{p \in \mathcal{C}_{\tau_k}\}, \Delta_k^{(i)} \mathbb{1}\{p \in \mathcal{C}_{\tau_k}\}$**

423 **Lemma 5.** *With a probability greater than  $1 - \frac{\delta}{12T^{5/4}}$ , we have that*

$$\begin{aligned} \sum_{k=1}^K \mathbb{1}\{p \in \mathcal{C}_{\tau_k}\} \Delta_k^{(R)} &\leq O(g(T))S \left( \sqrt{2} + 1 \right) \sqrt{AT \log \left( \frac{T}{\delta} \right)} + O(g(T)) \sqrt{2T \cdot \frac{5}{4} \log \left( \frac{8T(M+1)}{\delta} \right)} \\ &\quad + O(g(T)) S A \log \left( \frac{8T}{SA} \right) + \frac{T}{g(T)}, \end{aligned}$$

and

$$\begin{aligned} \sum_{k=1}^K \mathbb{1}\{p \in \mathcal{C}_{\tau_k}\} \Delta_k^{(i)} &\leq O(g(T))S \left( \sqrt{2} + 1 \right) \sqrt{AT \log \left( \frac{T}{\delta} \right)} + O(g(T)) \sqrt{2T \cdot \frac{5}{4} \log \left( \frac{8T(M+1)}{\delta} \right)} \\ &\quad + O(g(T)) S A \log \left( \frac{8T}{SA} \right) + \frac{T}{g(T)}, \forall i \in [1, M]. \end{aligned}$$

424 *Proof.* Since  $\mathbb{1}\{p \in \mathcal{C}_{\tau_k}\} \Delta_k^{(R)} = \Delta_{k,1}^{(R)} + \Delta_{k,2}^{(R)} + \Delta_{k,3}^{(R)}$ , proof follows by combining the bounds  
 425 derived in Lemma 2, Lemma 3 and Lemma 4. Similarly for  $\sum_k \Delta_k^{(i)} \mathbb{1}\{p \in \mathcal{C}_{\tau_k}\}$ .  $\square$

426 *Proof of Theorem 1.* Recall the regret decomposition result (34),

$$\Delta_k^{(R)} = \Delta_k^{(R)} \mathbb{1}\{p \notin \mathcal{C}_{\tau_k}\} + \Delta_k^{(R)} \mathbb{1}\{p \in \mathcal{C}_{\tau_k}\}, \quad (54)$$

$$\Delta_k^{(i)} = \Delta_k^{(i)} \mathbb{1}\{p \notin \mathcal{C}_{\tau_k}\} + \Delta_k^{(i)} \mathbb{1}\{p \in \mathcal{C}_{\tau_k}\}, \forall i \in [1, M]. \quad (55)$$

427 Substituting the upper-bounds for  $\sum_k \Delta_k^{(R)} \mathbb{1}\{p \notin \mathcal{C}_{\tau_k}\}, \sum_k \Delta_k^{(i)} \mathbb{1}\{p \notin \mathcal{C}_{\tau_k}\}$  derived in Lemma 1,  
 428 and the bound on  $\sum_k \Delta_k^{(R)} \mathbb{1}\{p \in \mathcal{C}_{\tau_k}\}, \sum_k \Delta_k^{(i)} \mathbb{1}\{p \in \mathcal{C}_{\tau_k}\}$  derived in Lemma 5, and utilizing the  
 429 union bound, we infer that the following bounds hold true in a set that has a probability greater than  
 430  $1 - \frac{2\delta}{12T^{5/4}}$ ,

$$\begin{aligned} \Delta^{(R)}(T) &\leq \sqrt{T} + O(g(T))S \left( \sqrt{2} + 1 \right) \sqrt{AT \log \left( \frac{T}{\delta} \right)} + O(g(T)) \sqrt{2T \cdot \frac{5}{4} \log \left( \frac{8T(M+1)}{\delta} \right)} \\ &\quad + O(g(T)) S A \log \left( \frac{8T}{SA} \right) + \frac{T}{g(T)}, \end{aligned}$$

and

$$\begin{aligned} \Delta^{(i)}(T) &\leq \sqrt{T} + O(g(T)) S \left( \sqrt{2} + 1 \right) \sqrt{AT \log \left( \frac{T}{\delta} \right)} + O(g(T)) \sqrt{2T \cdot \frac{5}{4} \log \left( \frac{8T(M+1)}{\delta} \right)} \\ &\quad + O(g(T)) S A \log \left( \frac{8T}{SA} \right) + \frac{T}{g(T)}, \\ &\quad \forall i \in [1, M]. \end{aligned}$$

431 The third term in the above bounds can be upper-bounded by  $O(g(T))S\sqrt{AT}\log\left(\frac{T}{\delta}\right)$ . The proof is  
 432 then completed by substituting this into the above bounds.  $\square$

## 433 B Proof of Theorem 2

### 434 B.1 Preliminary Results

435 We begin by deriving some results on the variations in the value of optimal reward of the CMDP (2)-  
 436 (3) as a function of the cost budgets  $c^{ub} = \{c_i^{ub}\}_{i=1}^M$ . Consider a vector  $\hat{c}^{ub} = \{\hat{c}_i^{ub}\}_{i=1}^M$  of cost  
 437 budgets that satisfies

$$c_i^{ub} - \epsilon \leq \hat{c}_i^{ub} \leq c_i^{ub}, \forall i \in [1, M], \quad (56)$$

438 where  $\epsilon > 0$ . Now consider the following CMDP in which the upper-bounds on the average costs are  
 439 equal to  $\{\hat{c}_i^{ub}\}_{i=1}^M$ .

$$\max_{\pi} \liminf_{T \rightarrow \infty} \frac{1}{T} \mathbb{E}_{\pi} \sum_{t=1}^T r(s_t, a_t) \quad (57)$$

$$\text{s.t. } \limsup_{T \rightarrow \infty} \frac{1}{T} \mathbb{E}_{\pi} \sum_{t=1}^T c_i(s_t, a_t) \leq \hat{c}_i^{ub}, i \in [1, M]. \quad (58)$$

440 **Lemma 6.** *Let the MDP  $p$  satisfy Assumption 1 and Assumption 2. Let  $\lambda^* = \{\lambda_i^*\}_{i=1}^M$  be an optimal  
 441 dual variable/Lagrange multiplier associated with the CMDP (57)-(58). Then,  $\lambda^*$  satisfies*

$$\sum_{i=1}^M \lambda_i^* \leq \frac{\hat{\eta}}{\eta},$$

442 where the constant  $\eta$  is as in (21), while  $\hat{\eta}$  is defined as follows,

$$\hat{\eta} := \max_{(s,a) \in \mathcal{S} \times \mathcal{A}} r(s, a) - \min_{(s,a) \in \mathcal{S} \times \mathcal{A}} r(s, a). \quad (59)$$

443 *Proof.* Within this proof, we let  $\pi^*(\hat{c}^{ub})$  denote an optimal stationary policy for (57)-(58). Recall  
 444 that the policy  $\pi_{feas.}$  that was defined in Assumption 2 satisfies  $\bar{c}_i(\pi_{feas.}) \leq c_i^{ub} - \eta$ . We have

$$\begin{aligned} \max_{(s,a) \in \mathcal{S} \times \mathcal{A}} r(s, a) &\geq \bar{r}(\pi^*(\hat{c}^{ub})) \\ &= \bar{r}(\pi^*(\hat{c}^{ub})) + \sum_{i=1}^M \lambda_i^* (\hat{c}_i^{ub} - \bar{c}_i(\pi^*(\hat{c}^{ub}))) \\ &\geq \bar{r}(\pi_{feas.}) + \sum_{i=1}^M \lambda_i^* (\hat{c}_i^{ub} - \bar{c}_i(\pi_{feas.})) \\ &\geq \min_{(s,a) \in \mathcal{S} \times \mathcal{A}} r(s, a) + \sum_{i=1}^M \lambda_i^* (\hat{c}_i^{ub} - \bar{c}_i(\pi_{feas.})) \\ &\geq \min_{(s,a) \in \mathcal{S} \times \mathcal{A}} r(s, a) + \eta \sum_{i=1}^M \lambda_i^*, \end{aligned}$$

445 where the second inequality follows since a policy that is optimal for the problem (57)-(58) maximizes  
 446 the Lagrangian  $\bar{r}(\pi) + \sum_{i=1}^M \lambda_i (\hat{c}_i^{ub} - \bar{c}_i(\pi))$  when the Lagrange multiplier  $\{\lambda_i\}_{i=1}^M$  is set equal to  
 447  $\{\lambda_i^*\}_{i=1}^M$  [Ber97]. Rearranging the above inequality yields the desired result.  $\square$

448 **Lemma 7.** *Let the MDP  $p$  satisfy Assumption 1 and Assumption 2. If  $r^*(\hat{c}^{ub})$  denotes optimal reward  
 449 value of (57), (58), and  $r^*$  is optimal reward of problem (2)-(3), then we have that*

$$r^* - r^*(\hat{c}^{ub}) \leq \left( \max_{i \in [1, M]} \{c_i^{ub} - \hat{c}_i^{ub}\} \right) \frac{\hat{\eta}}{\eta},$$

450 where  $\hat{\eta}$  is as in (59), and  $\eta$  is as in (21).

451 *Proof.* As discussed in Section 2.1, a CMDP can be posed as an LP. Since under Assumption 2, both  
 452 the CMDPs (2)-(3) and (57)-(58) are strictly feasible, we can use the strong duality property of LPs  
 453 [Ber97] in order to conclude that the optimal value of the primal and the dual problems for both the  
 454 CMDPs are equal. Thus,

$$r^* = \sup_{\pi} \inf_{\lambda} \bar{r}(\pi) + \sum_{i=1}^M \lambda_i (c_i^{ub} - \bar{c}_i(\pi)), \quad (60)$$

$$r^*(\hat{c}^{ub}) = \sup_{\pi} \inf_{\lambda} \bar{r}(\pi) + \sum_{i=1}^M \lambda_i (\hat{c}_i^{ub} - \bar{c}_i(\pi)). \quad (61)$$

455 Let  $\pi^{(1)}, \pi^{(2)}$  and  $\lambda^{(1)}, \lambda^{(2)}$  denote optimal policies and vector consisting of optimal dual variables  
 456 for the two CMDPs. It then follows from (60) and (61) that,

$$\begin{aligned} r^* &\leq \bar{r}(\pi^{(1)}) + \sum_{i=1}^M \lambda_i^{(2)} (c_i^{ub} - \bar{c}_i(\pi^{(1)})), \\ \text{and } r^*(\hat{c}^{ub}) &\geq \bar{r}(\pi^{(1)}) + \sum_{i=1}^M \lambda_i^{(2)} (\hat{c}_i^{ub} - \bar{c}_i(\pi^{(1)})). \end{aligned}$$

457 Subtracting the second inequality from the first yields

$$\begin{aligned} r^* - r^*(\hat{c}^{ub}) &\leq \sum_{i=1}^M \lambda_i^{(2)} (c_i^{ub} - \hat{c}_i^{ub}) \\ &\leq \left( \max_{i \in [1, M]} \{c_i^{ub} - \hat{c}_i^{ub}\} \right) \left( \sum_{i=1}^M \lambda_i^{(2)} \right) \\ &\leq \left( \max_{i \in [1, M]} \{c_i^{ub} - \hat{c}_i^{ub}\} \right) \frac{\hat{\eta}}{\eta}, \end{aligned}$$

458 where the last inequality in the above follows from Lemma 6. This completes the proof.  $\square$

## 459 B.2 Proof of Theorem 2

460 The proof is similar to the proof of Theorem 1; hence we only discuss the modifications required in  
 461 the proof of Theorem 1.

462 Since the construction of confidence bounds in the modified UCRL-CMDP remains the  
 463 same as in UCRL-CMDP, regret analysis for the case when confidence intervals fail,  
 464 i.e.,  $\{p \notin \mathcal{C}_{\tau_k}\}$ , remains the same as in proof of Theorem 1. Thus, the quantities  
 465  $\sum_{k=1}^K \Delta_k^{(R)} \{p \notin \mathcal{C}_{\tau_k}\}$ ,  $\sum_{k=1}^K \Delta_k^{(i)} \{p \notin \mathcal{C}_{\tau_k}\}$   $i = 1, 2, \dots, M$  can be upper-bounded similarly as  
 466 in Lemma 1.

467 The regret analysis on the set  $\{p \in \mathcal{C}_{\tau_k}\}$  undergoes the following changes. Inequalities (35), and (36)  
 468 are now modified as follows

$$r_k^* \geq r^* - \max_{i \in [1, M]} \{d_i\} \left( \frac{\hat{\eta}}{\eta} \right), \quad (62)$$

$$\text{and } c_{i,k}^* \leq c_i^{ub} - d_i, \forall i \in [1, M]. \quad (63)$$

469 They are derived using Lemma 7. It then follows from the modified bounds (62)-  
 470 (63) that the upper-bound (47) on  $\Delta_{k,1}^{(R)}$  now also constitutes an extra additive term  
 471 of  $\sum_{s,a} n_k(s, a) \max_i \{d_i\} \left( \frac{\hat{\eta}}{\eta} \right)$ ; while the bound on  $\Delta_{k,1}^{(i)}$  contains an additional term



472  $-d_i \sum_{s,a} n_k(s, a)$ . After summing up these bounds over episodes  $k$ , we obtain the following,

$$\begin{aligned} \sum_{k=1}^K \Delta_{k,1}^{(R)} &\leq (\sqrt{2} + 1)O(g(T))\sqrt{SAT} + \max_i (34 - b_i) \cdot \left(\frac{\hat{\eta}}{\eta}\right) \cdot O(g(T)) S \sqrt{A T \log\left(\frac{T}{\delta}\right)}, \text{ and} \\ \sum_{k=1}^K \Delta_{k,1}^{(i)} &\leq (\sqrt{2} + 1)O(g(T))\sqrt{SAT} - (34 - b_i) \cdot O(g(T)) S \sqrt{A T \log\left(\frac{T}{\delta}\right)}, \forall i \in [1, M]. \end{aligned} \quad (64)$$

473 The upper-bounds on  $\Delta_{k,2}^{(R)}, \Delta_{k,2}^{(i)}$  derived in Lemma 3 remain unchanged. Utilizing modified  
474 bounds (64), and proceeding along the same lines as in proof of Theorem 1 yields the desired  
475 result.

## 476 C Proof of Theorem 3

### 477 C.1 Preliminary Results

478 We begin by stating some preliminary results that will be utilized in the proof of Theorem 3.

479 **Lemma 8.** *Consider the dual problem (26) associated with the CMDP (2), (3), and let  $\lambda^*$  be a*  
480 *solution of the dual problem. If Assumption 2 holds true, then we have that*

$$\mathcal{D}(\lambda^*) = r^*, \quad (65)$$

481 where  $r^*$  is the optimal reward of CMDP (2), (3).

482 *Proof.* Under Assumption 2, the CMDP (2)-(3) is strictly feasible, so that Slater's constraint [BV04]  
483 is satisfied, and consequently strong duality holds true. Thus, if  $\lambda^*$  solves the dual problem (26), we  
484 then have that

$$\mathcal{D}(\lambda^*) = r^*. \quad (66)$$

485 □

486 **Lemma 9.** *Let  $\lambda = \{\lambda_i\}_{i=1}^M$  satisfy  $\lambda \geq \mathbf{0}$  and  $\phi$  be a learning algorithm for the problem of*  
487 *maximizing cumulative rewards under average cost constraints. We then have the following,*

$$\mathbb{E}_\phi \sum_{t=1}^T \left\{ r(s_t, a_t) + \sum_{i=1}^M \lambda_i (c_i^{ub} - c_i(s_t, a_t)) \right\} = r^* T - \mathbb{E}_\phi \Delta^{(R)}(T) - \sum_{i=1}^M \lambda_i \mathbb{E}_\phi \Delta^{(i)}(T). \quad (67)$$

488 *Proof.* We have,

$$\begin{aligned} \mathbb{E}_\phi \sum_{t=1}^T \left\{ r(s_t, a_t) + \sum_{i=1}^M \lambda_i (c_i^{ub} - c_i(s_t, a_t)) \right\} &= \mathbb{E}_\phi \sum_{t=1}^T r(s_t, a_t) + \sum_{i=1}^M \lambda_i \mathbb{E}_\phi \sum_{t=1}^T (c_i^{ub} - c_i(s_t, a_t)) \\ &= r^* T - \left( r^* T - \mathbb{E}_\phi \sum_{t=1}^T r(s_t, a_t) \right) - \sum_{i=1}^M \lambda_i \mathbb{E}_\phi \sum_{t=1}^T (c_i(s_t, a_t) - c_i^{ub}) \\ &= r^* T - \mathbb{E}_\phi \Delta^{(R)}(T) - \sum_{i=1}^M \lambda_i \mathbb{E}_\phi \Delta^{(i)}(T). \end{aligned}$$

489 □

### 490 C.2 Proof of Theorem 3

491 *Proof.* We begin by considering an auxiliary reward maximization problem that involves the  
492 same MDP  $p$ , but in which the reward received at time  $t$  by the agent is equal to  $r(s_t, a_t) +$   
493  $\sum_{i=1}^M \lambda_i (c_i(s_t, a_t) - c_i^{ub})$  instead of  $r(s_t, a_t)$ . However, there are no average cost constraints  
494 in the auxiliary problem. Let  $\phi'$  be a history dependent policy for this auxiliary problem. Denote its

optimal reward by  $r^*(\lambda)$ . Then, the regret for cumulative rewards collected by  $\phi'$  in the auxiliary problem is given by

$$r^*(\lambda) T - \mathbb{E}_{\phi'} \left[ \sum_{t=1}^T r(s_t, a_t) + \sum_{i=1}^M \lambda_i (c_i(s_t, a_t) - c_i^{ub}) \right].$$

It follows from Theorem 5 of [JOA10] that the controlled transition probabilities  $p(s, a, s')$  of the underlying MDP can be chosen so that this regret is greater than  $.015 \cdot \sqrt{D(p)SAT}$ , i.e.,

$$r^*(\lambda) T - \mathbb{E}_{\phi'} \left[ \sum_{t=1}^T r(s_t, a_t) + \sum_{i=1}^M \lambda_i (c_i(s_t, a_t) - c_i^{ub}) \right] \geq .015 \cdot \sqrt{D(p)SAT}. \quad (68)$$

We observe that any valid learning algorithm for the constrained problem is also a valid algorithm for the auxiliary problem. Thus, if  $\phi$  is a learning algorithm for the problem with average cost constraints, then we have

$$r^*(\lambda) T - \mathbb{E}_{\phi} \left[ \sum_{t=1}^T r(s_t, a_t) + \sum_{i=1}^M \lambda_i (c_i(s_t, a_t) - c_i^{ub}) \right] \geq .015 \cdot \sqrt{D(p)SAT}. \quad (69)$$

We now substitute (67) in the above to obtain

$$\mathbb{E}_{\phi} \Delta^{(R)}(T) + \sum_{i=1}^M \lambda_i \mathbb{E}_{\phi} \Delta^{(i)}(T) \geq .015 \cdot \sqrt{D(p)SAT} + r^*T - r^*(\lambda) T. \quad (70)$$

Since the expression in the r.h.s. is maximized for values of  $\lambda$  which are optimal for the dual problem (26), we set it equal to  $\lambda^*$ , and then use Lemma 8 in order to obtain

$$\mathbb{E}_{\phi} \Delta^{(R)}(T) + \sum_{i=1}^M \lambda_i \mathbb{E}_{\phi} \Delta^{(i)}(T) \geq .015 \cdot \sqrt{D(p)SAT}. \quad (71)$$

This completes the proof.  $\square$

## D Some Auxiliary Results

### D.1 Augmented CMDP

Consider the problem (14)-(17) that involves solving for an optimistic MDP, and the corresponding optimal policy. We repeat it below for the convenience of readers,

$$\begin{aligned} & \max_{\mu, p'} \sum_{(s,a) \in \mathcal{S} \times \mathcal{A}} \mu(s, a) r(s, a), \\ & \text{s.t.} \sum_{a \in \mathcal{A}} \mu(s, a) = \sum_{(s', b) \in \mathcal{S} \times \mathcal{A}} \mu(s', b) p'(s', b, s), \\ & \sum_{(s,a) \in \mathcal{S} \times \mathcal{A}} \mu(s, a) c_i(s, a) \leq c_i^{ub}, i \in [1, M] \\ & \mu(s, a) \geq 0 \quad \forall (s, a) \in \mathcal{S} \times \mathcal{A}, \quad \sum_{(s,a) \in \mathcal{S} \times \mathcal{A}} \mu(s, a) = 1, \\ & p' \in \mathcal{C}_{\tau_k}, \end{aligned}$$

where  $\mathcal{C}_{\tau_k}$  denotes the confidence interval associated with the estimate  $\hat{p}_{\tau_k}$ .

Now consider an equivalent ‘‘augmented’’ CMDP, one in which the decision  $a_t^{(+)}$  at each time  $t$  comprises of the following two quantities:

(i) the action  $a_t$  corresponding to the control input that has to be applied to the original MDP, and also,

(ii) the MDP  $p_t$ , i.e., the controlled transition probabilities  $p_t \in \mathcal{C}_{\tau_k}$ .

The state and action-spaces for this augmented CMDP are given by  $\mathcal{S}$  and  $\mathcal{A} \times \mathcal{C}_{\tau_k}$  respectively. We

denote by  $\pi^{(+)}$  a policy that makes decisions for the augmented CMDP. The augmented CMDP is described as follows,

$$\max_{\pi^{(+)}} \liminf_{T \rightarrow \infty} \frac{1}{T} \mathbb{E}_{\pi^{(+)}} \sum_{t=1}^T r(s_t, a_t^{(+)}) \quad (72)$$

$$\text{s.t. } \limsup_{T \rightarrow \infty} \frac{1}{T} \mathbb{E}_{\pi^{(+)}} \sum_{t=1}^T c_i(s_t, a_t^{(+)}) \leq c_i^{ub}, i \in [1, M]. \quad (73)$$

We let  $\mu^{(+)} \in \Delta(\mathcal{S} \times \mathcal{A} \times \mathcal{C}_{\tau_k})$  denote an occupation measure for the augmented problem. This CMDP can be posed as an infinite LP in which the decision variable is the occupation measure  $\mu^{(+)}$ . An optimal policy can be obtained by solving this infinite LP, similar to the LP scheme discussed in Section 2. Approximation schemes for an infinite LP can be found in [HLL98, HLGHL03].

## D.2 Ergodicity of the Process $s_t$

The following result is a standard tool from the theory of perturbation analysis of Markov chains.

**Lemma 10.** (*Perturbations of Markov Chains*) Consider two finite-state Markov chains evolving on a state-space  $\mathcal{S}$ , with transition probabilities described by  $\{P(i, j)\}_{i, j \in \mathcal{S}}$  and  $\{\tilde{P}(i, j)\}_{i, j \in \mathcal{S}}$ . If  $\pi$  and  $\tilde{\pi}$  denote their stationary distributions, we then have that

$$\tilde{\pi} - \pi = \tilde{\pi} (\tilde{P} - P) (I - P + \mathbf{1}\pi^T)^{-1}.$$

*Proof.* See [Pau68].

**Lemma 11.** Consider a finite-state controlled Markov process  $s_t$  that evolves according to transition probabilities  $\sum_{a \in \mathcal{A}} \pi(a|s)p(s, a, s')$ , and receives a reward equal to  $r(s_t, a_t)$  at time  $t$ . Let  $P^t(i, j)$  denote the probability of a  $t$ -step transition from state  $i$  to state  $j$ , and let  $P^\infty$  denote the stationary distribution. Let  $t_0 \in \mathbb{N}$  be such that  $\min_{i, j \in \mathcal{S}} P^{t_0}(i, j) > 0$ , and define

$$\rho := \min_{i, j} P^{t_0}(i, j). \quad (74)$$

Then, the following statements are true.

1.

$$\|P^t(s, \cdot) - P^\infty(\cdot)\| \leq (1 - \rho)^{\lfloor t/t_0 \rfloor}, \quad (75)$$

where for  $x \in \mathbb{R}$ ,  $\lfloor x \rfloor$  denotes the greatest integer less than or equal to  $x$ . Moreover, the limiting value of the average expected reward  $\lim_{T \rightarrow \infty} \frac{1}{T} \sum_{t=1}^T \sum_{x \in \mathcal{S}} P^t(s, x) \pi(a|x) r(x, a)$ , where  $\pi(a|x)$  denotes the probability with which  $\pi$  chooses action  $a$  when the state is  $s$ , does not depend upon the initial state  $s$ .

2. There exists a function  $v_\pi^{(R)} : \mathcal{S} \times \mathcal{A} \mapsto \mathbb{R}$  which satisfies the following,

$$\bar{r}(\pi) + v_\pi^{(R)}(s) = \sum_{a \in \mathcal{A}} \pi(a|s) r(s, a) + \sum_{a \in \mathcal{A}} \sum_{s' \in \mathcal{S}} \pi(a|s) p(s, a, s') v_\pi^{(R)}(s'), \forall s \in \mathcal{S}, \quad (76)$$

where  $\bar{r}(\pi)$  denotes the average reward under  $\pi$ . Moreover,

$$|v_\pi^{(R)}(s)| \leq \max_{(s, a)} r(s, a) \frac{t_0}{1 - \rho}, \forall s \in \mathcal{S}. \quad (77)$$

There also exist functions  $v_\pi^{(i)}, i \in [1, M]$  that have similar properties.

*Proof.* 1. The process  $s_t$  is a finite-state Markov chain, and hence necessarily ergodic [S. 12]. Proof of (75) follows from Doeblin's coupling; refer to page 38 of [Tor02] for a detailed proof. The result that the limiting average reward does not depend upon the initial state, follows from (75).

544 To see 2.), let  $J_n(s)$  denote the expected value of the total reward collected by the policy  $\pi$  when the  
 545 system starts in state  $s$ , and operates for  $n$  time-steps. We have the following recursive relation,

$$J_n(s) = \sum_{a \in \mathcal{A}} \pi(a|s) r(s, a) + \sum_{a \in \mathcal{A}} \pi(a|s) \sum_{s' \in \mathcal{S}} p(s, a, s') J_{n-1}(s'), \forall s \in \mathcal{S}. \quad (78)$$

546 Consider the following,

$$J_n(s) = n\bar{r}(\pi) + j_n(s), \forall s \in \mathcal{S},$$

547 where

$$j_n(s) = \mathbb{E}_\pi \left( \sum_{t=1}^n r(s_t, a_t) - \bar{r}(\pi) \middle| s_0 = s \right). \quad (79)$$

548 We show that  $j_n$  converges as  $n \rightarrow \infty$ , and moreover we identify  $v_\pi^{(R)}$  with this limit. Substituting  
 549 the expression (79) into (78), we obtain the following,

$$\bar{r}(\pi) + j_n(s) = \sum_{a \in \mathcal{A}} \pi(a|s) r(s, a) + \sum_{a \in \mathcal{A}} \pi(a|s) \sum_{s' \in \mathcal{S}} p(s, a, s') j_{n-1}(s'), \forall s \in \mathcal{S}. \quad (80)$$

550 Let  $j_n := \{j_n(s)\}_{s \in \mathcal{S}}$  be the vector consisting of differential cost-to-go functions. Note that

$$j_n(s) = \sum_{t=1}^n \left( \sum_{s'} P^t(s, s') \sum_a \pi(a|s') r(s', a) - P^\infty(s') \sum_a \pi(a|s') r(s', a) \right). \quad (81)$$

551 By substituting the bounds derived in 1. into the above inequality, we conclude that the sequence  
 552 of vectors  $j_n$  is Cauchy, and hence has a limit. We denote this limit as  $\{v^{(R)}(s)\}_{s \in \mathcal{S}}$ . Since  $j_n(\cdot)$   
 553 satisfy the recursion (80), the limit  $v^{(R)}(\cdot)$  also satisfies the same. This proves (76).

554 (77) follows by substituting the inequality derived in 1. into (81).  $\square$

555  $\bar{p}_k = \{\bar{p}_k(s, a, s') : s, s' \in \mathcal{S}, a \in \mathcal{A}\}$ : We define  $\bar{p}_k$  as follows. Recall that  $\tilde{p}_k$  is the controlled  
 556 transition probability obtained by solving the problem (14)-(17). Let  $p_{rand.}$  denote the controlled  
 557 transition probability of an MDP that is drawn uniformly at random from the confidence set  $\mathcal{C}_{\tau_k}$  ( $\tau_k$   
 558 denotes the time when the  $k$ -th episode begins). With a probability  $(1 - \gamma_t)$ ,  $\bar{p}_k$  assumes the value  
 559  $\tilde{p}_k$ , i.e., the dynamics of the MDP are governed by the solution of the LP (14)-(17). However, with a  
 560 probability  $\gamma_t$ ,  $\bar{p}_k$  is equal to  $p_{rand.}$ . The following result discusses the ergodicity properties of the  
 561 process whose evolution is governed by  $\bar{p}_k$ .

562 **Lemma 12.** *Let  $\tilde{s}_t$  be a controlled Markov process in which the control transition probabilities are*  
 563 *equal to  $\bar{p}_k$ , while the controls are generated according to  $\tilde{\pi}_k$ . Then, the following are true:*

564 1. *Let  $\bar{r}(SR(\tilde{\mu}_k))$  denote the reward obtained by applying controls according to  $SR(\tilde{\mu}_k)$  on*  
 565 *the MDP with control transition probabilities equal to  $\bar{p}_k$ . Its average reward is greater*  
 566 *than or equal to  $\bar{r}(SR(\tilde{\mu}_k)) - O(\gamma_t)$ . Similarly, its  $i$ -th average cost is less than or equal*  
 567 *to  $\bar{c}_i(SR(\tilde{\mu}_k)) + O(\gamma_t)$ .*

568 2. *The conclusions of 2. Lemma 11 hold true. Moreover,*

$$|v_\pi^{(R)}(s)|, |v_\pi^{(i)}(s)| \leq 1/O(\gamma_{\tau_k}), \forall s \in \mathcal{S}. \quad (82)$$

569 *Proof.* 1. is a direct consequence of Lemma 10. To prove 2., it suffices to show that the assumptions  
 570 of Lemma 11 hold true. More precisely, the existence of a  $t_0 \in \mathbb{N}$  for which (74) holds true. However,  
 571 since w.p.  $\gamma_t$ , we have that the control transition probabilities are chosen uniformly at random from  
 572 the set  $\mathcal{C}_{\tau_k}$ , this means that all the controlled transitions  $(s, a) \rightarrow s'$  have a probability that is atleast  
 573  $O(\gamma_t)$ . This shows the existence of a desired  $t_0$ . Moreover, we have that the quantity  $\rho$  defined as  
 574 in (74) satisfies  $\rho \geq O(\gamma_t)$ . The proof then follows from Lemma 11.  $\square$
